# Supplementary material for: Distilling Self-Supervised Vision Transformers for Weakly-Supervised Few-Shot Classification & Segmentation
Source: arXiv:2307.03407 source file (2023-07-07)
Supplement: Supplementary file 1 [file gfss.tex]

\begin{table}[!t]
	\small
	% \vspace{-3mm}
	\centering
    \scalebox{0.95}{
	{
		\begin{tabular}{ 
				l  c |
				c c c c
				 }
			\toprule
             & 
            & \multicolumn{2}{c}{1-shot}
			& \multicolumn{2}{c}{5-shot}  \\
            model & supervision & base & novel & base & novel \\
			% &\multicolumn{2}{c}{1-shot (base/novel)} 
			% &\multicolumn{2}{c}{5-shot (base/novel)}  
			% \specialrule{0em}{0pt}{1pt}			
			% \cline{4-7}
			% \specialrule{0em}{1pt}{0pt}			
			
			% model & gFSS & supervision
			% & base  & novel 
			% & base  & novel \\
			
			\specialrule{0em}{0pt}{1pt}
			\hline
			\specialrule{0em}{1pt}{0pt}
			
			% PANet~[69] & \xmark & pixel-level & 31.9 / 11.3 & 33.0 / 15.3 \\

			CAPL~\cite{tian2020generalized} & pixel-level
			& 65.5 & 18.9
			& 66.1 & 22.4  \\ 			

 			\multirow{2}{*}{CST (ours)} & image-level
			& 20.0 & 28.7
			& 26.9 & 33.5  \\ 	
   
    		& pixel-level 
			& 40.0 & 50.3
			& 51.4 & 58.9  \\ 	
			\bottomrule      			                             
		\end{tabular}
	}
 }
	\caption{
 Comparing segmentation mIoU (\%) for generalized few-shot segmentation (GFS-Seg) on Pascal-5$^{i}$.}	
	\label{table:gfss}   	
	\vspace{-3mm}
\end{table}
